# Supplementary material for: A Large-scale Dataset for Hate Speech Detection on Vietnamese Social Media Texts
Source: arXiv:2103.11528 source file (2021-07-20)
Supplement: Supplementary file 1 [file appendix.tex]

\appendix
\section{Appendix}
\label{appendix}
In this section, we described some difficult comments that annotators are confused about in the annotation process. Those comments have three different labels by three different annotators. Table \ref{tab_confused_comments} shows confused comments.

\begin{center}
    \begin{longtable}{|C{0.5cm}|p{4.1cm}|p{7.1cm}|}
    \caption{Difficult comments that confuse the annotators in the UIT-HSD dataset}
     \label{tab_confused_comments} \\
        \hline
        \textbf{\#} & \makecell[c]{\textbf{Comments}} & \makecell[c]{\textbf{Description}} \\
        \hline
    %   1 & \makecell*[{{p{4cm}}}]{Tụi t đéo nịnh tụi t thương cô vì tánh cô chân thật. M biết cái cc gì m nói (\textit{English: We do not flatter her. We love her because she is very friendly. You f*cking know nothing to say that.}) } & \makecell*[{{p{7cm}}}]{This comment contained offensive words such as: \textit{"đéo"},  \textit{"cc"}. However, \textit{"đéo"} in Vietnamese is slang, and in some context, it does not contain negative meaning. Besides, \textit{"cc"} is an abbreviation, which has different meaning based on the annotators' thinking. Thus, it is difficult to determine the label for that comment.} \\
    %   \hline
       1 & \makecell*[{{p{4cm}}}]{T đang nhìn clgv (\textit{English: What the f*ck i am watching at})} & \makecell*[{{p{7cm}}}]{The phrase \textit{clgv} is an abbreviation, and it usually appeared on many comments of users on social network sites. In some case, it does not contains hate. However, in some annotators viewpoint, the phrase \textit{clgv} has a profane meaning.} \\ 
       \hline
      2 & \makecell*[{{p{4cm}}}]{Thân lăm bây giò lại căn buôi nhau (\textit{English: They are very friendly before. Now they swallow d*ck each other})} & \makecell*[{{p{7cm}}}]{This comment has an implicit phrase: \textit{căn buôi nhau}. It is an offensive word phrase in Vietnamese; however, does not directly denote. Also, the word \textit{buôi} in Vietnamese have a profane meaning.} \\
      \hline
    %   4 & \makecell*[{{p{6cm}}}]{Sản phẩm chất lượng để phục vụ một lũ \textit{“cực kỳ thuyết phục”} bị di căn giai đoạn cuối quả phí phạm. Toàn bọn bại não, thoái hoá văn hoá. Cứ tưởng thế là hay ho. \\ (\textit{English: This is for bastard gangs named "cực kỳ thuyết phục", who are Cerebral Palsy, clumsy, and dummy. But they always think that they are wise and smart.}) } & \makecell*[{{p{5.2cm}}}]{The phrase "cực kỳ thuyết phục" is an unusual phrase that only appears in the social network, and are used widely by teenagers to blame a specific group of people on the social network.} \\
    %   \hline
      3 & \makecell*[{{p{4cm}}}]{Game cu lon nay =))) (\textit{English: What is a pussy game !!})} & \makecell*[{{p{7cm}}}]{This comment is written in Vietnamese without accents.  Thus, it confuses annotators.} \\
      \hline
    %   6 & \makecell*[{{p{4.5cm}}}]{Anh cút cm luôn hộ em cái (\textit{English: Get out of my sight!}) } & \makecell*[{{p{6.5cm}}}]{This comments have the offensive word \textit{"cm"}, which means \textit{"got damn"} in English, however, is written in abbreviation form. Besides, this comment seems to be humour than harassment. Thus, this comment confuses annotators.}  \\
    %   \hline
    %   7 & \makecell*[{{p{6cm}}}]{Con lợn này béo vãi lon. Bắp tay to bằng ngón chân =)) \\ (\textit{English: This woman is so fat. The arm is as big as the leg.}) } & \makecell*[{{p{5.2cm}}}]{This comment has a figurative meaning. The word \textit{"Con lợn này"} refers to a specific person in Vietnamese. The phrase \textit{"Bắp tay to bằng ngón chân"} imply the characteristic of a person in bad meaning.} \\
    %   \hline
      
    \end{longtable}
\end{center}
